# Supplementary material for: MVS2D: Efficient Multi-view Stereo via Attention-Driven 2D Convolutions
Source: arXiv:2104.13325 source file (2021-12-11)
Supplement: Supplementary file 1 [file 07_supp.tex]

\section{Details of Experiments}
\subsection{Model Details}
We use ResNet-18 (with the fully connected layer and pooling layer removed) as the building block of our networks $\set{G}$ and $\set{F}$. $\set{F}$ additionally includes two up-sampling and convolution layer that output a feature map $F_0 \in \mathcal{R}^{\frac{h}{4}\times \frac{w}{4}\times c}$, where $h$ and $w$ are the input image's height and width respectively. $F_0$ is further feed into a small network with 3 convolutions and 3 de-convolutions to recover a depth probability volume $F_1\in \set{R}^{\frac{h}{4}\times \frac{w}{4}\times k'}$. $F_1$ is finally decoded into a depth map $d_{\frac{1}{4}}\in \mathcal{R}^{\frac{h}{4}\times \frac{w}{4}}$ using the soft-argmax operation as in MVSNet~\cite{yao2018mvsnet}. To supervise the network at full resolution instead of $\frac{1}{4}$ resolution, we further upsample $d_{\frac{1}{4}}$ to the full resolution via nearest interpolation, and add a predicted residual to it to get final prediction $d \in \mathcal{R}^{h\times w}$. Please refer to our released code for more details. %We included our code in the supplementary materials.

\begin{table*}[!ht]
\centering
\resizebox{0.9\textwidth}{!}{%
\begin{tabular}{r|ccccc|ccc}
\toprule
\multicolumn{1}{c|}{Method}       & AbsRel $\downarrow$ & AbsDiff $\downarrow$& SqRel $\downarrow$& RMSE $\downarrow$  & RMSELog $\downarrow$& $\delta<1.25$ $\uparrow$& $\delta<1.25^2$ $\uparrow$& $\delta<1.25^3$ $\uparrow$ \\ \hline

COLMAP &  0.384  &   0.843  &   1.26  &    1.480  &    0.500  &   0.482 &  0.663 & 0.840\\ % no conf
DeMoN &0.311& 1.330& 19.970& 2.607& 0.247& 0.641 &0.902 &0.967\\
DeepMVS  &0.231  &0.663  &0.615 & 1.149  &0.302 & 0.674 & 0.887  &0.941\\
DPSNet  &0.081 &0.201 &0.097 &0.442 &0.160 &0.885& 0.945& 0.973\\
NAS  &\textbf{0.068} &\textbf{0.168}& \textbf{0.056}& 0.375& 0.142 &\textbf{0.905} &0.964 &0.988\\
\hline
Ours-robust &   0.100   & 0.231 &   0.057   &   \textbf{0.313}  &  \textbf{0.140}  &   0.895  &   \textbf{0.966}  &   \textbf{0.991}\\
 Ours & 0.108  &   0.271 & 0.130   &   0.513 &  0.184 &   0.860  &   0.939  &   0.973  \\
\bottomrule
\end{tabular}
}
\caption{Depth evaluation results on the MVS dataset (trained on RGBD, SUN3D, and Scenes11). Please see Sec.~\ref{supp:sec2.4} for discussion.}
\label{table:generalization1}
\end{table*}

\begin{table*}[!ht]
\centering
\resizebox{0.9\textwidth}{!}{%
\begin{tabular}{r|ccccc|ccc}
\toprule
\multicolumn{1}{c|}{Method}       & AbsRel $\downarrow$ & SqRel $\downarrow$& log10 $\downarrow$& RMSE $\downarrow$  & RMSELog $\downarrow$& $\delta<1.25$ $\uparrow$& $\delta<1.25^2$ $\uparrow$& $\delta<1.25^3$ $\uparrow$ \\ \hline
MVSNet  & 0.154  &   0.125  &   0.067  &   0.478  &   0.212  &   0.779  & 0.927  &   0.973  \\
NAS  & 0.134  &   0.094  &   0.064  &   0.434  &   0.190  &   0.789  &  0.932  &   0.979  \\
\hline
Ours &  \textbf{0.113}  &   \textbf{0.062}  &   \textbf{0.049}  &   \textbf{0.332}  &   \textbf{0.149}  &   \textbf{0.871}  &   \textbf{0.968} &  \textbf{0.993} \\
Ours-robust &  0.115  &   0.066  &   0.052  &   0.354  &   0.158  &   0.862  &   0.960 & 0.990\\ 
\bottomrule
\end{tabular}
}
\caption{Depth evaluation results on the SUN3D dataset (trained on ScanNet). Please see Sec.~\ref{supp:sec2.4} for discussion. }
\label{table:generalization2}
\end{table*}

\subsection{Training Details} We use 4 NVIDIA DGX-V100 GPUs with 32GB memory each to conduct following experiments. 

\noindent\textbf{ScanNet.}
We train for 30 epochs with a batch size 16, and reduce the learning rate by 10 at epoch 25 and 28. The input image size is $640\times 480$.  During training, we sample depth hypothesis uniformly in inverse depth space
\begin{equation}
    d_i = 1/((1 - \frac{i}{k})\frac{1}{d_{\text{min}}} + \frac{i}{k} \frac{1}{d_{\text{max}}}),
\end{equation}
where $k$ is the number of depth hypothesis. We set $k=32$,  $d_{\text{min}} = 0.3$, and $d_{\text{max}} = 10.1$.

We trained several baselines on ScanNet dataset. Specifically, we trained MVSNet~\cite{yao2018mvsnet} for 500k iterations. We trained FastMVSNet~\cite{yu2020fast} for a total 30 epochs, with the last 10 epochs optimizing the GaussNewton layer. We trained NAS~\cite{kusupati2019normal} for 20 epochs for initialization, and 10 epoch including the normal consistency module. We trained PatchmatchNet~\cite{wang2021patchmatchnet} for 30 epochs. We trained DPSNet~\cite{im2019dpsnet} for 20 epochs. We trained Bts~\cite{lee2019big} for 20 epochs. The training for MVSNet/DPSNet costs around 3 days. The training for NAS costs around 5 days. The training time of FastMVSNet/PatchmatchNet costs around 1 day.  

\noindent\textbf{SUN3D, RGBD, and Scenes11.} We follow similar setup as the training of ScanNet. During training, we sample depth hypothesis uniformly in inverse depth space:  
\begin{equation}
d_i = 1/((1 - \frac{i}{k})\frac{1}{d_{\text{min}}} + \frac{i}{k} \frac{1}{d_{\text{max}}}),
\end{equation}
where $d_{\text{min}} = 0.5$, $d_{\text{max}} = 32.0$.

\noindent\textbf{DTU.}
One modification we made on training DTU dataset is that we add a confidence prediction. The added confidence will be used to filter out unconfident predictions during the final 3D reconstruction. We adopt following loss~\cite{kendall2017uncertainties}:

\begin{equation}
    \mathcal{L} = \frac{|\hat{d} - d_{\text{gt}}|}{\hat{\sigma} } + \log(\hat{\sigma}),
\end{equation}
where $\hat{\sigma}$ is the predicted confidence map. We implement this confidence prediction by adding a separate head in the final output. Such confidence prediction is trained along with depth prediction without the need for explicit supervision. During the test time, we set a threshold $\tau$ for $\hat{\sigma}$ and prune all predictions $\hat{d_i}$ whose corresponding $\hat{\sigma_i}$ are larger than $\tau$.

We train for 80 epochs with a batch size 8, and reduce the learning rate by ten at epoch 40 and 70. The input image size is $1536\times 1152$. The training takes around 5 days. We follow the practice of the robust training scheme \cite{wang2021patchmatchnet} and use randomly chosen 4 reference images for each source image during training. We use $N=96$ depth hypothesis uniformly sampled in the inverse depth space ($d_i = 1/((1 - \frac{i}{k})\frac{1}{d_{\text{min}}} + \frac{i}{k} \frac{1}{d_{\text{max}}})$. We use $d_{\text{min}} = 425.0$, $d_{\text{max}} = 935.0$. During testing, we use top 4 reference images(ranked by a heuristic criterior introduced in ~\cite{yao2018mvsnet}), which is the same as previous approaches~\cite{yao2018mvsnet,chen2019point,wang2021patchmatchnet}. We fuse the depth maps into final 3D model using the fusion code provided in ~\cite{wang2021patchmatchnet}. The qualitative results on DTU test set can be found in Figure \ref{fig:visualization:dtu}. 

\subsection{Speed Comparison} 
We use one V100 GPU to conduct the speed benchmark for all methods. to We feed each method an input image of size 640x480. For methods that do not produce full-resolution depth maps (i.e. MVSNet~\cite{yao2018mvsnet}), we further up-sampled them to the full resolution using nearest-neighbor interpolation. The FPS numbers are averaged over 500 random inputs for each method.

\subsection{Pose Corruption} 

We use the following procedure to generate perturbations for input poses. Assume the ground truth relative pose is $T=[R\, |\, t]$ between the source image and a certain reference image.  Firstly, we sample $N$ points $\{p_k\}_{k=1}^{N}$ on corresponding ground-truth 3D point cloud of the source image. We use $N=10$ in our experiments. Then, we project those $N$ points into reference image using ground truth relative pose $T$ and camera intrinsics $\mathcal{K}$ to get $\{\overline{p}_k\}_{k=1}^{N}$. We then perturb $\{\overline{p}_k\}_{k=1}^{N}$  by adding  noise from a uniform distribution whose maximum value is 10 pixels. We solve a $\text{PnP}$ problem~\cite{andrew2001multiple} using $\{p_k\}_{k=1}^{N}$ and the perturbed pixels $\{\overline{p}_k\}_{k=1}^{N}$ to get the corrupted $\overline{T}=[\overline{R}\, |\, \overline{t}]$. We accept the perturbed $\overline{T}$ if the average pixel offset over the source image is less than 10 pixels. Otherwise, we set $\overline{T} = T$. We pre-compute all perturbations for all image pairs. Figure~\ref{fig:perturb_hist} shows the statistics of pose perturbations. Specifically, we plot the histogram of $\Delta R = \arccos(\frac{\Tr(\overline{R}R^{-1})-1}{2})$, and $\Delta t=\norm{\overline{t} - t}_2$.

\begin{figure}[!h]
\includegraphics[trim=30 0 30 20,clip,width=0.49\linewidth]{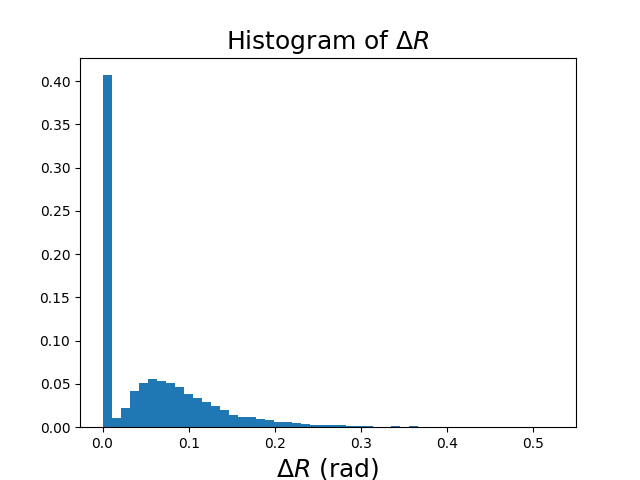}
\includegraphics[trim=30 0 30 20,clip,width=0.49\linewidth]{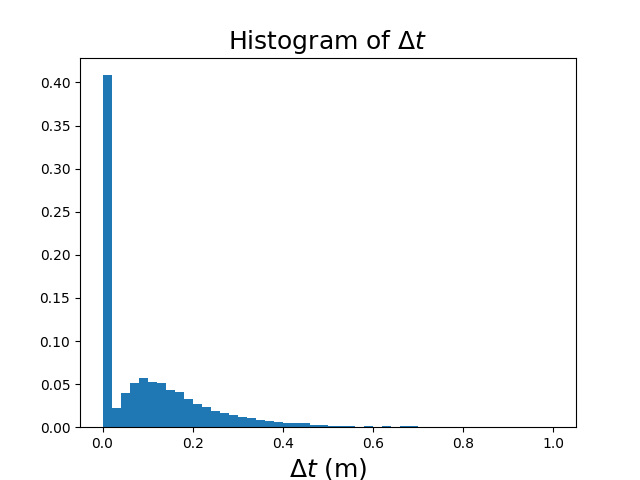}
\caption{Pose corruption statistics. Left: histogram of rotation perturbation. Right: histogram of translation perturbation.}
\label{fig:perturb_hist}
\vspace{-0.1in}
\end{figure}

\section{Additional Studies}

\subsection{Generalization Ability}
\label{supp:sec2.4}
We did two experiments to evaluate the generalization ability of all methods to unseen datasets. Following the experimental setups of DeMoN and NAS, we use the model trained on SUN3D/RGBD/Scenes11 and test on the MVS dataset, which is an outdoor dataset and the data distributions are very different from the training set. The results can be found in Table~\ref{table:generalization1}. Our methods perform better than COLMAP, DeMoN and DeepMVS, although they still fall behind 
NAS under some metrics such as $AbsRel$. Such a result is reasonable since our approach is better adapted to the training distribution, which will lead to performance drop on heavily out-of-distribution test data. 

To further examine each method's performance on unseen datasets whose input data statistics are similar to those in the training sets, we further test models trained using ScanNet on SUN3D test sets (see Table~\ref{table:generalization2}). The input data of SUN3D ScanNet are all indoor scenes. We can see that our methods still perform favorably among other methods. 

\subsection{Ablation Study on Mask Encoding}
\label{supp:sec2.5}
To study the benefits of mask encoding, we further experiment with \textbf{Ours-nomask} which removes the mask encoding in Eq 5.
The results on ScanNet can be found in Table \ref{table:ablation_mask}. Remove mask encoding (\textbf{Ours-nomask}) leads to worse results than \textbf{Ours}.  Such behavior is reasonable since mask encoding provides an easy way for the network to distinguish the valid and invalid interpolation, thus facilitate the training.

\begin{table}[!ht]
\centering
\resizebox{0.46\textwidth}{!}{%
\begin{tabular}{r|cccc}
\toprule
\multicolumn{1}{c|}{Method}       & AbsRel $\downarrow$ & $\delta<1.25$ $\uparrow$& $thre@0.2$ $\uparrow$ & $thre@0.5$ $\uparrow$\\ \hline
Ours-nomask &  0.0605 & 0.9635 & 0.8543  & 0.9719\\ 
Ours &  \textbf{0.0597}   & \textbf{0.9640}  & \textbf{0.8585} & \textbf{0.9735}\\ 
\bottomrule
\end{tabular}
}
\caption{Ablation study on mask encoding. $thre@0.2$/$thre@0.5$ measures the percentage of pixel that has absolute depth error less than 0.2m/0.5m respectively. Removing mask encoding hurts the performance, especially for \textit{AbsRel}} 
\label{table:ablation_mask}
\end{table}

\subsection{More Qualitative Results}
We show additional visualizations of depth predictions in Figure~\ref{fig:qualitative1}~\&~\ref{fig:qualitative2}. Our method produces higher quality depth estimations compared to other MVS methods and performs better than one of the state-of-the-art single-view depth estimation method Bts. Additionally, we show more qualitative comparisons on 3D reconstruction in Figure \ref{fig:supp_3drecon}. Our method generates comparable or even better visual results with other methods that require expensive 3D convolutions. We also show the reconstruction result on DTU test set in Figure \ref{fig:visualization:dtu}.

\newpage

\begin{figure*}
\newcommand{\TT}[1]{\raisebox{-0.5\height}{#1}}
\setlength{\tabcolsep}{1pt}
\footnotesize
\def\imw{0.14\textwidth}
\begin{tabular}{ccccccc}

Bts & MVSNet & FastMVSNet & DPSNet & NAS & MVS2D (Ours) & G.T.  \\

\TT{\includegraphics[width=\imw]{Figures/Figure3_jet/scene0011_00-0080_0079_0081/bts.png}} & 
\TT{\includegraphics[width=\imw]{Figures/Figure3_jet/scene0011_00-0080_0079_0081/mvsnet.png}} & 
\TT{\includegraphics[width=\imw]{Figures/Figure3_jet/scene0011_00-0080_0079_0081/fastmvsnet.png}} & 
\TT{\includegraphics[width=\imw]{Figures/Figure3_jet/scene0011_00-0080_0079_0081/dpsnet.png}} & 
\TT{\includegraphics[width=\imw]{Figures/Figure3_jet/scene0011_00-0080_0079_0081/nas.png}} & 
\TT{\includegraphics[width=\imw]{Figures/Figure3_jet/scene0011_00-0080_0079_0081/ours.png}} & 
\TT{\includegraphics[width=\imw]{Figures/Figure3_jet/scene0011_00-0080_0079_0081/gt.png}}  \\

\TT{\includegraphics[width=\imw]{Figures/Figure3_jet/scene0025_01-0045_0044_0046/bts.png}} & 
\TT{\includegraphics[width=\imw]{Figures/Figure3_jet/scene0025_01-0045_0044_0046/mvsnet.png}} & 
\TT{\includegraphics[width=\imw]{Figures/Figure3_jet/scene0025_01-0045_0044_0046/fastmvsnet.png}} & 
\TT{\includegraphics[width=\imw]{Figures/Figure3_jet/scene0025_01-0045_0044_0046/dpsnet.png}} & 
\TT{\includegraphics[width=\imw]{Figures/Figure3_jet/scene0025_01-0045_0044_0046/nas.png}} & 
\TT{\includegraphics[width=\imw]{Figures/Figure3_jet/scene0025_01-0045_0044_0046/ours.png}} & 
\TT{\includegraphics[width=\imw]{Figures/Figure3_jet/scene0025_01-0045_0044_0046/gt.png}}  \\

\TT{\includegraphics[width=\imw]{Figures/Figure3_jet/scene0030_01-0075_0074_0076/bts.png}} & 
\TT{\includegraphics[width=\imw]{Figures/Figure3_jet/scene0030_01-0075_0074_0076/mvsnet.png}} & 
\TT{\includegraphics[width=\imw]{Figures/Figure3_jet/scene0030_01-0075_0074_0076/fastmvsnet.png}} & 
\TT{\includegraphics[width=\imw]{Figures/Figure3_jet/scene0030_01-0075_0074_0076/dpsnet.png}} & 
\TT{\includegraphics[width=\imw]{Figures/Figure3_jet/scene0030_01-0075_0074_0076/nas.png}} & 
\TT{\includegraphics[width=\imw]{Figures/Figure3_jet/scene0030_01-0075_0074_0076/ours.png}} & 
\TT{\includegraphics[width=\imw]{Figures/Figure3_jet/scene0030_01-0075_0074_0076/gt.png}}  \\

\TT{\includegraphics[width=\imw]{Figures/Figure3_jet/scene0046_01-0011_0010_0012/bts.png}} & 
\TT{\includegraphics[width=\imw]{Figures/Figure3_jet/scene0046_01-0011_0010_0012/mvsnet.png}} & 
\TT{\includegraphics[width=\imw]{Figures/Figure3_jet/scene0046_01-0011_0010_0012/fastmvsnet.png}} & 
\TT{\includegraphics[width=\imw]{Figures/Figure3_jet/scene0046_01-0011_0010_0012/dpsnet.png}} & 
\TT{\includegraphics[width=\imw]{Figures/Figure3_jet/scene0046_01-0011_0010_0012/nas.png}} & 
\TT{\includegraphics[width=\imw]{Figures/Figure3_jet/scene0046_01-0011_0010_0012/ours.png}} & 
\TT{\includegraphics[width=\imw]{Figures/Figure3_jet/scene0046_01-0011_0010_0012/gt.png}}  \\

\TT{\includegraphics[width=\imw]{Figures/Figure3_jet/scene0050_00-0001_0000_0002/bts.png}} & 
\TT{\includegraphics[width=\imw]{Figures/Figure3_jet/scene0050_00-0001_0000_0002/mvsnet.png}} & 
\TT{\includegraphics[width=\imw]{Figures/Figure3_jet/scene0050_00-0001_0000_0002/fastmvsnet.png}} & 
\TT{\includegraphics[width=\imw]{Figures/Figure3_jet/scene0050_00-0001_0000_0002/dpsnet.png}} & 
\TT{\includegraphics[width=\imw]{Figures/Figure3_jet/scene0050_00-0001_0000_0002/nas.png}} & 
\TT{\includegraphics[width=\imw]{Figures/Figure3_jet/scene0050_00-0001_0000_0002/ours.png}} & 
\TT{\includegraphics[width=\imw]{Figures/Figure3_jet/scene0050_00-0001_0000_0002/gt.png}}  \\

\TT{\includegraphics[width=\imw]{Figures/Figure3_jet/scene0064_01-0033_0032_0034/bts.png}} & 
\TT{\includegraphics[width=\imw]{Figures/Figure3_jet/scene0064_01-0033_0032_0034/mvsnet.png}} & 
\TT{\includegraphics[width=\imw]{Figures/Figure3_jet/scene0064_01-0033_0032_0034/fastmvsnet.png}} & 
\TT{\includegraphics[width=\imw]{Figures/Figure3_jet/scene0064_01-0033_0032_0034/dpsnet.png}} & 
\TT{\includegraphics[width=\imw]{Figures/Figure3_jet/scene0064_01-0033_0032_0034/nas.png}} & 
\TT{\includegraphics[width=\imw]{Figures/Figure3_jet/scene0064_01-0033_0032_0034/ours.png}} & 
\TT{\includegraphics[width=\imw]{Figures/Figure3_jet/scene0064_01-0033_0032_0034/gt.png}}  \\

\TT{\includegraphics[width=\imw]{Figures/Figure3_jet/scene0187_01-0090_0089_0091/bts.png}} & 
\TT{\includegraphics[width=\imw]{Figures/Figure3_jet/scene0187_01-0090_0089_0091/mvsnet.png}} & 
\TT{\includegraphics[width=\imw]{Figures/Figure3_jet/scene0187_01-0090_0089_0091/fastmvsnet.png}} & 
\TT{\includegraphics[width=\imw]{Figures/Figure3_jet/scene0187_01-0090_0089_0091/dpsnet.png}} & 
\TT{\includegraphics[width=\imw]{Figures/Figure3_jet/scene0187_01-0090_0089_0091/nas.png}} & 
\TT{\includegraphics[width=\imw]{Figures/Figure3_jet/scene0187_01-0090_0089_0091/ours.png}} & 
\TT{\includegraphics[width=\imw]{Figures/Figure3_jet/scene0187_01-0090_0089_0091/gt.png}}  \\

\TT{\includegraphics[width=\imw]{Figures/Figure3_jet/scene0088_00-0007_0006_0008/bts.png}} & 
\TT{\includegraphics[width=\imw]{Figures/Figure3_jet/scene0088_00-0007_0006_0008/mvsnet.png}} & 
\TT{\includegraphics[width=\imw]{Figures/Figure3_jet/scene0088_00-0007_0006_0008/fastmvsnet.png}} & 
\TT{\includegraphics[width=\imw]{Figures/Figure3_jet/scene0088_00-0007_0006_0008/dpsnet.png}} & 
\TT{\includegraphics[width=\imw]{Figures/Figure3_jet/scene0088_00-0007_0006_0008/nas.png}} & 
\TT{\includegraphics[width=\imw]{Figures/Figure3_jet/scene0088_00-0007_0006_0008/ours.png}} & 
\TT{\includegraphics[width=\imw]{Figures/Figure3_jet/scene0088_00-0007_0006_0008/gt.png}}  \\

\TT{\includegraphics[width=\imw]{Figures/Figure3_jet/scene0100_02-0039_0038_0040/bts.png}} & 
\TT{\includegraphics[width=\imw]{Figures/Figure3_jet/scene0100_02-0039_0038_0040/mvsnet.png}} & 
\TT{\includegraphics[width=\imw]{Figures/Figure3_jet/scene0100_02-0039_0038_0040/fastmvsnet.png}} & 
\TT{\includegraphics[width=\imw]{Figures/Figure3_jet/scene0100_02-0039_0038_0040/dpsnet.png}} & 
\TT{\includegraphics[width=\imw]{Figures/Figure3_jet/scene0100_02-0039_0038_0040/nas.png}} & 
\TT{\includegraphics[width=\imw]{Figures/Figure3_jet/scene0100_02-0039_0038_0040/ours.png}} & 
\TT{\includegraphics[width=\imw]{Figures/Figure3_jet/scene0100_02-0039_0038_0040/gt.png}}  \\

\TT{\includegraphics[width=\imw]{Figures/Figure3_jet/scene0050_01-0128_0127_0129/bts.png}} & 
\TT{\includegraphics[width=\imw]{Figures/Figure3_jet/scene0050_01-0128_0127_0129/mvsnet.png}} & 
\TT{\includegraphics[width=\imw]{Figures/Figure3_jet/scene0050_01-0128_0127_0129/fastmvsnet.png}} & \TT{\includegraphics[width=\imw]{Figures/Figure3_jet/scene0050_01-0128_0127_0129/dpsnet.png}} & 
\TT{\includegraphics[width=\imw]{Figures/Figure3_jet/scene0050_01-0128_0127_0129/nas.png}} & 
\TT{\includegraphics[width=\imw]{Figures/Figure3_jet/scene0050_01-0128_0127_0129/ours.png}} & 
\TT{\includegraphics[width=\imw]{Figures/Figure3_jet/scene0050_01-0128_0127_0129/gt.png}}  \\

\TT{\includegraphics[width=\imw]{Figures/Figure3_jet/scene0064_00-0014_0013_0015/bts.png}} & 
\TT{\includegraphics[width=\imw]{Figures/Figure3_jet/scene0064_00-0014_0013_0015/mvsnet.png}} & 
\TT{\includegraphics[width=\imw]{Figures/Figure3_jet/scene0064_00-0014_0013_0015/fastmvsnet.png}} & \TT{\includegraphics[width=\imw]{Figures/Figure3_jet/scene0064_00-0014_0013_0015/dpsnet.png}} & 
\TT{\includegraphics[width=\imw]{Figures/Figure3_jet/scene0064_00-0014_0013_0015/nas.png}} & 
\TT{\includegraphics[width=\imw]{Figures/Figure3_jet/scene0064_00-0014_0013_0015/ours.png}} & 
\TT{\includegraphics[width=\imw]{Figures/Figure3_jet/scene0064_00-0014_0013_0015/gt.png}}  \\

\end{tabular}
\caption{[1/2] Qualitative results on depth prediction. Each row corresponds to one test example. The region without ground truth depth labels is colored white in the last column. Our prediction outperforms both the single-view depth estimation method and other multi-view methods. }
\label{fig:qualitative1}
\end{figure*}

\begin{figure*}
\newcommand{\TT}[1]{\raisebox{-0.5\height}{#1}}
\setlength{\tabcolsep}{1pt}
\footnotesize
\def\imw{0.14\textwidth}
\begin{tabular}{ccccccc}

Bts & MVSNet & FastMVSNet & DPSNet & NAS & MVS2D (Ours) & G.T. \\

\TT{\includegraphics[width=\imw]{Figures/Figure3_jet/scene0146_01-0018_0017_0019/bts.png}} & 
\TT{\includegraphics[width=\imw]{Figures/Figure3_jet/scene0146_01-0018_0017_0019/mvsnet.png}} & 
\TT{\includegraphics[width=\imw]{Figures/Figure3_jet/scene0146_01-0018_0017_0019/fastmvsnet.png}} & 
\TT{\includegraphics[width=\imw]{Figures/Figure3_jet/scene0146_01-0018_0017_0019/dpsnet.png}} & 
\TT{\includegraphics[width=\imw]{Figures/Figure3_jet/scene0146_01-0018_0017_0019/nas.png}} & 
\TT{\includegraphics[width=\imw]{Figures/Figure3_jet/scene0146_01-0018_0017_0019/ours.png}} & 
\TT{\includegraphics[width=\imw]{Figures/Figure3_jet/scene0146_01-0018_0017_0019/gt.png}} \\

\TT{\includegraphics[width=\imw]{Figures/Figure3_jet/scene0164_00-0075_0074_0076/bts.png}} & 
\TT{\includegraphics[width=\imw]{Figures/Figure3_jet/scene0164_00-0075_0074_0076/mvsnet.png}} & 
\TT{\includegraphics[width=\imw]{Figures/Figure3_jet/scene0164_00-0075_0074_0076/fastmvsnet.png}} & 
\TT{\includegraphics[width=\imw]{Figures/Figure3_jet/scene0164_00-0075_0074_0076/dpsnet.png}} & 
\TT{\includegraphics[width=\imw]{Figures/Figure3_jet/scene0164_00-0075_0074_0076/nas.png}} & 
\TT{\includegraphics[width=\imw]{Figures/Figure3_jet/scene0164_00-0075_0074_0076/ours.png}} & 
\TT{\includegraphics[width=\imw]{Figures/Figure3_jet/scene0164_00-0075_0074_0076/gt.png}} \\

\TT{\includegraphics[width=\imw]{Figures/Figure3_jet/scene0187_00-0004_0003_0005/bts.png}} & 
\TT{\includegraphics[width=\imw]{Figures/Figure3_jet/scene0187_00-0004_0003_0005/mvsnet.png}} & 
\TT{\includegraphics[width=\imw]{Figures/Figure3_jet/scene0187_00-0004_0003_0005/fastmvsnet.png}} & 
\TT{\includegraphics[width=\imw]{Figures/Figure3_jet/scene0187_00-0004_0003_0005/dpsnet.png}} & 
\TT{\includegraphics[width=\imw]{Figures/Figure3_jet/scene0187_00-0004_0003_0005/nas.png}} & 
\TT{\includegraphics[width=\imw]{Figures/Figure3_jet/scene0187_00-0004_0003_0005/ours.png}} & 
\TT{\includegraphics[width=\imw]{Figures/Figure3_jet/scene0187_00-0004_0003_0005/gt.png}} \\

\TT{\includegraphics[width=\imw]{Figures/Figure3_jet/scene0193_01-0003_0002_0004/bts.png}} & 
\TT{\includegraphics[width=\imw]{Figures/Figure3_jet/scene0193_01-0003_0002_0004/mvsnet.png}} & 
\TT{\includegraphics[width=\imw]{Figures/Figure3_jet/scene0193_01-0003_0002_0004/fastmvsnet.png}} & 
\TT{\includegraphics[width=\imw]{Figures/Figure3_jet/scene0193_01-0003_0002_0004/dpsnet.png}} & 
\TT{\includegraphics[width=\imw]{Figures/Figure3_jet/scene0193_01-0003_0002_0004/nas.png}} & 
\TT{\includegraphics[width=\imw]{Figures/Figure3_jet/scene0193_01-0003_0002_0004/ours.png}} & 
\TT{\includegraphics[width=\imw]{Figures/Figure3_jet/scene0193_01-0003_0002_0004/gt.png}} \\

\TT{\includegraphics[width=\imw]{Figures/Figure3_jet/scene0187_00-0084_0083_0085/bts.png}} & 
\TT{\includegraphics[width=\imw]{Figures/Figure3_jet/scene0187_00-0084_0083_0085/mvsnet.png}} & 
\TT{\includegraphics[width=\imw]{Figures/Figure3_jet/scene0187_00-0084_0083_0085/fastmvsnet.png}} & 
\TT{\includegraphics[width=\imw]{Figures/Figure3_jet/scene0187_00-0084_0083_0085/dpsnet.png}} & 
\TT{\includegraphics[width=\imw]{Figures/Figure3_jet/scene0187_00-0084_0083_0085/nas.png}} & 
\TT{\includegraphics[width=\imw]{Figures/Figure3_jet/scene0187_00-0084_0083_0085/ours.png}} & 
\TT{\includegraphics[width=\imw]{Figures/Figure3_jet/scene0187_00-0084_0083_0085/gt.png}} \\

\TT{\includegraphics[width=\imw]{Figures/Figure3_jet/scene0203_00-0019_0018_0020/bts.png}} & 
\TT{\includegraphics[width=\imw]{Figures/Figure3_jet/scene0203_00-0019_0018_0020/mvsnet.png}} & 
\TT{\includegraphics[width=\imw]{Figures/Figure3_jet/scene0203_00-0019_0018_0020/fastmvsnet.png}} & 
\TT{\includegraphics[width=\imw]{Figures/Figure3_jet/scene0203_00-0019_0018_0020/dpsnet.png}} & 
\TT{\includegraphics[width=\imw]{Figures/Figure3_jet/scene0203_00-0019_0018_0020/nas.png}} & 
\TT{\includegraphics[width=\imw]{Figures/Figure3_jet/scene0203_00-0019_0018_0020/ours.png}} & 
\TT{\includegraphics[width=\imw]{Figures/Figure3_jet/scene0203_00-0019_0018_0020/gt.png}} \\

\TT{\includegraphics[width=\imw]{Figures/Figure3_jet/scene0207_00-0010_0009_0011/bts.png}} & 
\TT{\includegraphics[width=\imw]{Figures/Figure3_jet/scene0207_00-0010_0009_0011/mvsnet.png}} & 
\TT{\includegraphics[width=\imw]{Figures/Figure3_jet/scene0207_00-0010_0009_0011/fastmvsnet.png}} & 
\TT{\includegraphics[width=\imw]{Figures/Figure3_jet/scene0207_00-0010_0009_0011/dpsnet.png}} & 
\TT{\includegraphics[width=\imw]{Figures/Figure3_jet/scene0207_00-0010_0009_0011/nas.png}} & 
\TT{\includegraphics[width=\imw]{Figures/Figure3_jet/scene0207_00-0010_0009_0011/ours.png}} & 
\TT{\includegraphics[width=\imw]{Figures/Figure3_jet/scene0207_00-0010_0009_0011/gt.png}} \\

\TT{\includegraphics[width=\imw]{Figures/Figure3_jet/scene0208_00-0003_0002_0004/bts.png}} & 
\TT{\includegraphics[width=\imw]{Figures/Figure3_jet/scene0208_00-0003_0002_0004/mvsnet.png}} & 
\TT{\includegraphics[width=\imw]{Figures/Figure3_jet/scene0208_00-0003_0002_0004/fastmvsnet.png}} & 
\TT{\includegraphics[width=\imw]{Figures/Figure3_jet/scene0208_00-0003_0002_0004/dpsnet.png}} & 
\TT{\includegraphics[width=\imw]{Figures/Figure3_jet/scene0208_00-0003_0002_0004/nas.png}} & 
\TT{\includegraphics[width=\imw]{Figures/Figure3_jet/scene0208_00-0003_0002_0004/ours.png}} & 
\TT{\includegraphics[width=\imw]{Figures/Figure3_jet/scene0208_00-0003_0002_0004/gt.png}} \\

\TT{\includegraphics[width=\imw]{Figures/Figure3_jet/scene0222_00-0012_0011_0013/bts.png}} & 
\TT{\includegraphics[width=\imw]{Figures/Figure3_jet/scene0222_00-0012_0011_0013/mvsnet.png}} & 
\TT{\includegraphics[width=\imw]{Figures/Figure3_jet/scene0222_00-0012_0011_0013/fastmvsnet.png}} & 
\TT{\includegraphics[width=\imw]{Figures/Figure3_jet/scene0222_00-0012_0011_0013/dpsnet.png}} & 
\TT{\includegraphics[width=\imw]{Figures/Figure3_jet/scene0222_00-0012_0011_0013/nas.png}} & 
\TT{\includegraphics[width=\imw]{Figures/Figure3_jet/scene0222_00-0012_0011_0013/ours.png}} & 
\TT{\includegraphics[width=\imw]{Figures/Figure3_jet/scene0222_00-0012_0011_0013/gt.png}} \\

\TT{\includegraphics[width=\imw]{Figures/Figure3_jet/scene0077_01-0046_0045_0044/bts.png}} & 
\TT{\includegraphics[width=\imw]{Figures/Figure3_jet/scene0077_01-0046_0045_0044/mvsnet.png}} & 
\TT{\includegraphics[width=\imw]{Figures/Figure3_jet/scene0077_01-0046_0045_0044/fastmvsnet.png}} & \TT{\includegraphics[width=\imw]{Figures/Figure3_jet/scene0077_01-0046_0045_0044/dpsnet.png}} & 
\TT{\includegraphics[width=\imw]{Figures/Figure3_jet/scene0077_01-0046_0045_0044/nas.png}} & 
\TT{\includegraphics[width=\imw]{Figures/Figure3_jet/scene0077_01-0046_0045_0044/ours.png}} & 
\TT{\includegraphics[width=\imw]{Figures/Figure3_jet/scene0077_01-0046_0045_0044/gt.png}}  \\

\TT{\includegraphics[width=\imw]{Figures/Figure3_jet/scene0095_01-0025_0024_0026/bts.png}} & 
\TT{\includegraphics[width=\imw]{Figures/Figure3_jet/scene0095_01-0025_0024_0026/mvsnet.png}} & 
\TT{\includegraphics[width=\imw]{Figures/Figure3_jet/scene0095_01-0025_0024_0026/fastmvsnet.png}} & \TT{\includegraphics[width=\imw]{Figures/Figure3_jet/scene0095_01-0025_0024_0026/dpsnet.png}} & 
\TT{\includegraphics[width=\imw]{Figures/Figure3_jet/scene0095_01-0025_0024_0026/nas.png}} & 
\TT{\includegraphics[width=\imw]{Figures/Figure3_jet/scene0095_01-0025_0024_0026/ours.png}} & 
\TT{\includegraphics[width=\imw]{Figures/Figure3_jet/scene0095_01-0025_0024_0026/gt.png}}  \\

\end{tabular}
\caption{[2/2] Qualitative results on depth prediction. Each row corresponds to one test example. The region without ground truth depth labels is colored white in the last column. Our prediction outperforms both the single-view depth estimation method and other multi-view methods. }
\label{fig:qualitative2}
\end{figure*}

\begin{figure*}
\newcommand{\TT}[1]{\raisebox{-0.5\height}{#1}}
\setlength{\tabcolsep}{1pt}
\footnotesize
\def\imw{0.2\textwidth}
\begin{tabular}{ccccc}
MVSNet &FastMVSNet  & DPSNet & NAS & MVS2D (Ours) \\

\TT{\includegraphics[width=\imw]{Figures/Figure4_new/scene0316_00/mvsnet.png}}
&\TT{\includegraphics[width=\imw]{Figures/Figure4_new/scene0316_00/fastmvsnet.png}} &
\TT{\includegraphics[width=\imw]{.igures/Figure4_new/scene0316_00/dpsnet.png}}  &
\TT{\includegraphics[width=\imw]{Figures/Figure4_new/scene0316_00/nas.png}} &
\TT{\includegraphics[width=\imw]{Figures/Figure4_new/scene0316_00/ours.png}} \\
\vspace{0.2in}
\TT{\includegraphics[width=\imw]{Figures/Figure4_new/scene0277_00/mvsnet.png}}
&\TT{\includegraphics[width=\imw]{Figures/Figure4_new/scene0277_00/fastmvsnet.png}} &
\TT{\includegraphics[width=\imw]{Figures/Figure4_new/scene0277_00/dpsnet.png}}  &
\TT{\includegraphics[width=\imw]{Figures/Figure4_new/scene0277_00/nas.png}} &
\TT{\includegraphics[width=\imw]{Figures/Figure4_new/scene0277_00/ours.png}} \\
\vspace{0.2in}
\TT{\includegraphics[width=\imw]{Figures/Figure4_new/scene0149_00/mvsnet.png}}
&\TT{\includegraphics[width=\imw]{Figures/Figure4_new/scene0149_00/fastmvsnet.png}} &
\TT{\includegraphics[width=\imw]{Figures/Figure4_new/scene0149_00/dpsnet.png}}  &
\TT{\includegraphics[width=\imw]{Figures/Figure4_new/scene0149_00/nas.png}} &
\TT{\includegraphics[width=\imw]{Figures/Figure4_new/scene0149_00/ours.png}} \\
\vspace{0.2in}
\TT{\includegraphics[width=\imw]{Figures/Figure4_new/scene0146_00/mvsnet.png}}
&\TT{\includegraphics[width=\imw]{Figures/Figure4_new/scene0146_00/fastmvsnet.png}} &
\TT{\includegraphics[width=\imw]{Figures/Figure4_new/scene0146_00/dpsnet.png}}  &
\TT{\includegraphics[width=\imw]{Figures/Figure4_new/scene0146_00/nas.png}} &
\TT{\includegraphics[width=\imw]{Figures/Figure4_new/scene0146_00/ours.png}} \\
\vspace{0.2in}
\TT{\includegraphics[width=\imw]{Figures/Figure4_new/scene0300_00/mvsnet.png}}
&\TT{\includegraphics[width=\imw]{Figures/Figure4_new/scene0300_00/fastmvsnet.png}} &
\TT{\includegraphics[width=\imw]{Figures/Figure4_new/scene0300_00/dpsnet.png}}  &
\TT{\includegraphics[width=\imw]{Figures/Figure4_new/scene0300_00/nas.png}} &
\TT{\includegraphics[width=\imw]{Figures/Figure4_new/scene0300_00/ours.png}} \\
\vspace{0.2in}
\TT{\includegraphics[width=\imw]{Figures/Figure4_new/scene0084_00/mvsnet.png}}
&\TT{\includegraphics[width=\imw]{Figures/Figure4_new/scene0084_00/fastmvsnet.png}} &
\TT{\includegraphics[width=\imw]{Figures/Figure4_new/scene0084_00/dpsnet.png}}  &
\TT{\includegraphics[width=\imw]{Figures/Figure4_new/scene0084_00/nas.png}} &
\TT{\includegraphics[width=\imw]{Figures/Figure4_new/scene0084_00/ours.png}} \\
\TT{\includegraphics[width=\imw]{Figures/Figure4_new/scene0488_00/mvsnet.png}}
&\TT{\includegraphics[width=\imw]{Figures/Figure4_new/scene0488_00/fastmvsnet.png}} &
\TT{\includegraphics[width=\imw]{Figures/Figure4_new/scene0488_00/dpsnet.png}}  &
\TT{\includegraphics[width=\imw]{Figures/Figure4_new/scene0488_00/nas.png}} &
\TT{\includegraphics[width=\imw]{Figures/Figure4_new/scene0488_00/ours.png}} \\
\TT{\includegraphics[width=\imw]{Figures/Figure4_new/scene0338_00/mvsnet.png}}
&\TT{\includegraphics[width=\imw]{Figures/Figure4_new/scene0338_00/fastmvsnet.png}} &
\TT{\includegraphics[width=\imw]{Figures/Figure4_new/scene0338_00/dpsnet.png}}  &
\TT{\includegraphics[width=\imw]{Figures/Figure4_new/scene0338_00/nas.png}} &
\TT{\includegraphics[width=\imw]{Figures/Figure4_new/scene0338_00/ours.png}} \\
\end{tabular}
\caption{Qualitative scene reconstruction results on ScanNet. Our method yields smoother outputs than other baselines. We zoom in parts of a scene (\textcolor{red}{red} box) and show at the corner (\textcolor{blue}{blue} box) to highlight the differences. Best viewed in PDF.} \label{fig:supp_3drecon}
\end{figure*}

\begingroup
\setlength{\tabcolsep}{1.0pt} % Default value: 6pt
   \begin{figure*}[!ht]
    \centering
    \hspace{-1em}
     \def\imw{0.28\textwidth}
     \def\imh{0.25\textheight}
     \def\fbox{}

     \begin{tabular}{ccc}
 \fbox{\includegraphics[trim={100 0 0 0},clip, height=\imh, width=\imw, keepaspectratio]{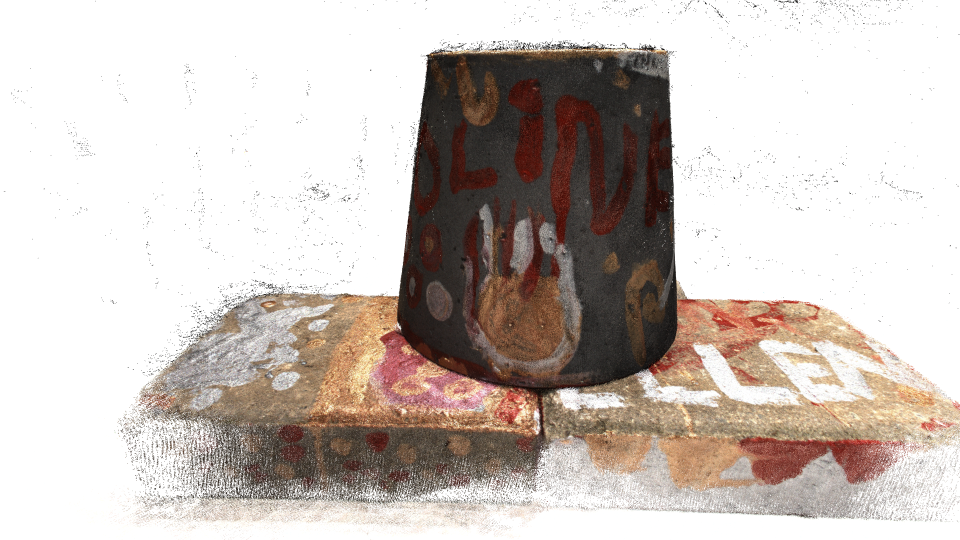}} &
        \fbox{\includegraphics[trim={200 100 200 0},clip,height=\imh, width=\imw, keepaspectratio]{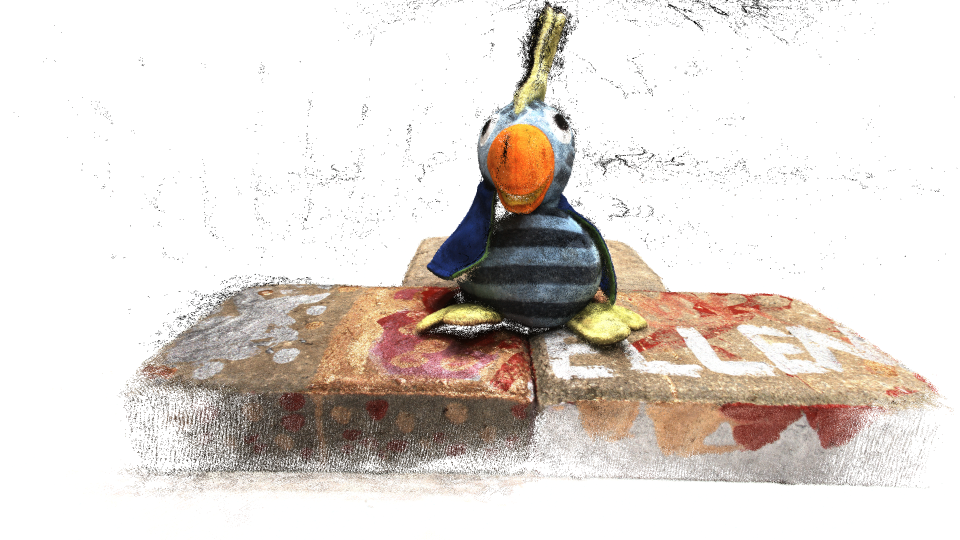}} & \fbox{\includegraphics[trim={400 100 400 200},clip,height=\imh, width=\imw, keepaspectratio]{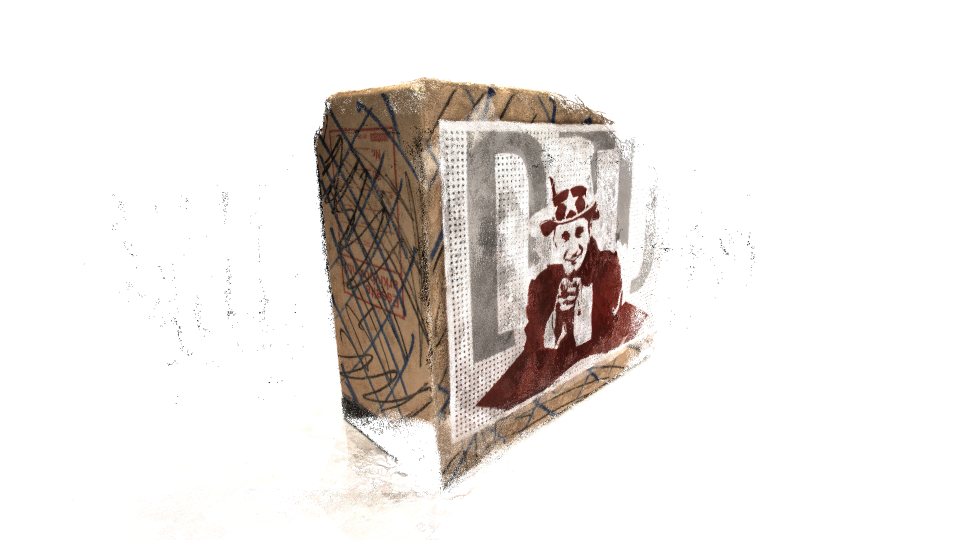}} \\ 
        \fbox{\includegraphics[trim={400 100 550 200},clip,height=\imh, width=\imw, keepaspectratio]{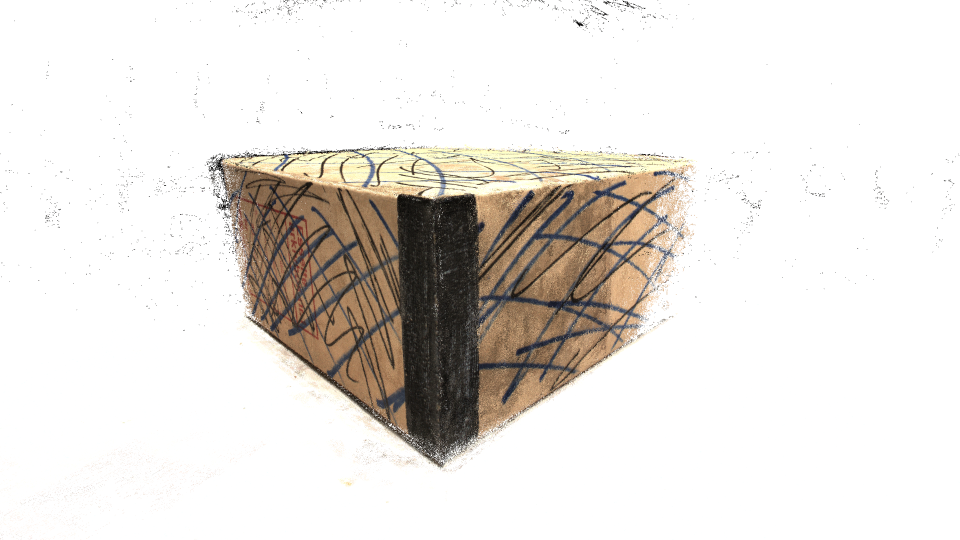}} & 
        \fbox{\includegraphics[trim={600 200 300 50},clip,height=\imh, width=\imw, keepaspectratio]{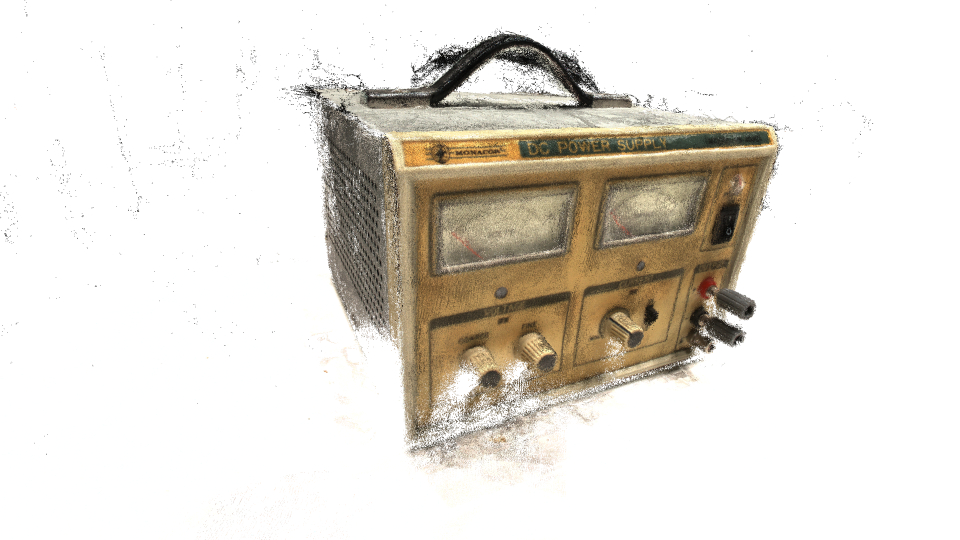}} & \fbox{\includegraphics[trim={300 100 200 0},clip,height=\imh, width=\imw, keepaspectratio]{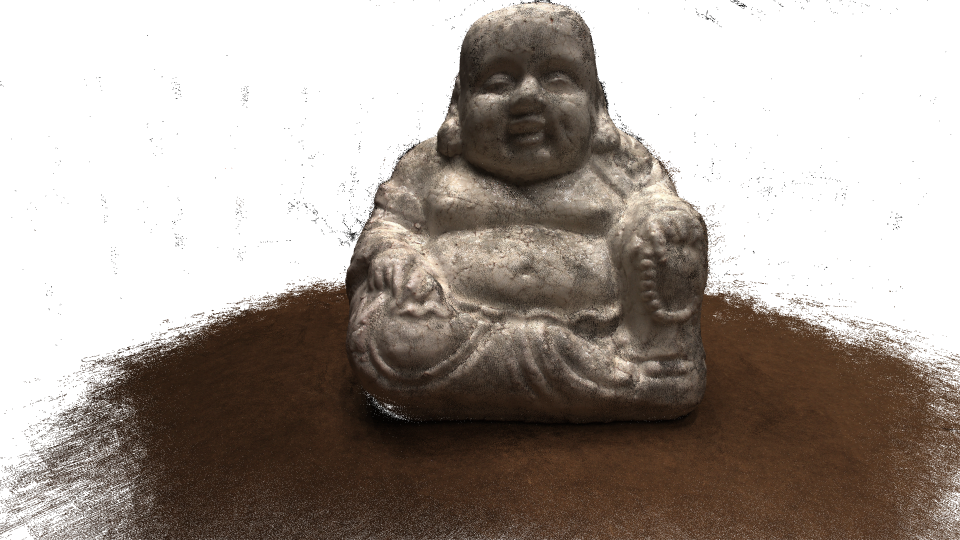}} \\
        \fbox{\includegraphics[trim={100 00 300 00},clip,height=\imh, width=\imw, keepaspectratio]{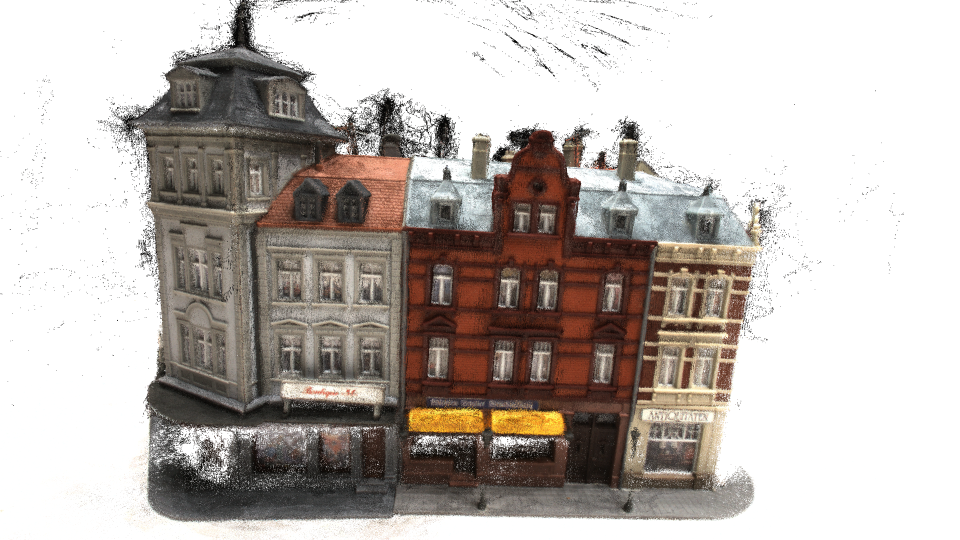}}  &
        \fbox{\includegraphics[trim={100 0 100 50},clip,height=\imh, width=\imw, keepaspectratio]{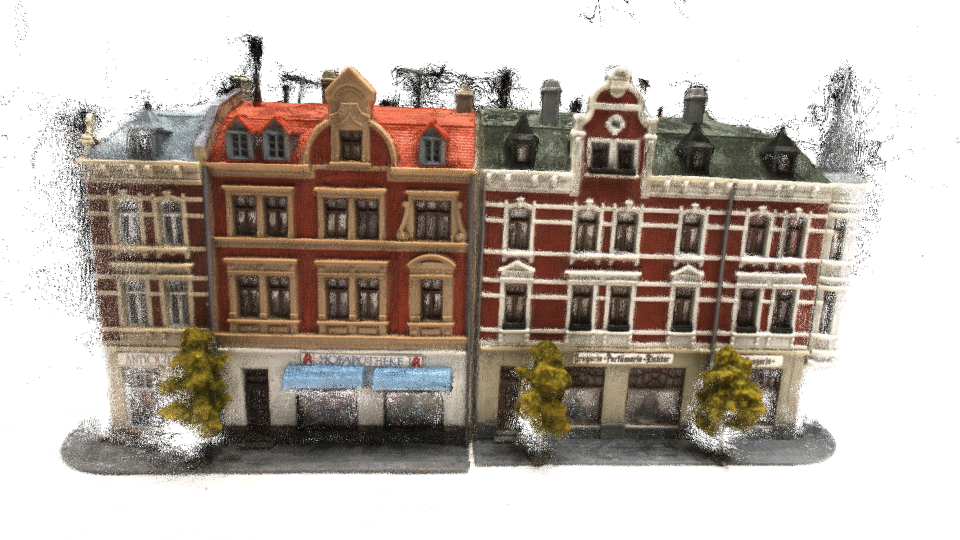}} &
        \fbox{\includegraphics[trim={00 0 00 0},clip,height=\imh, width=\imw, keepaspectratio]{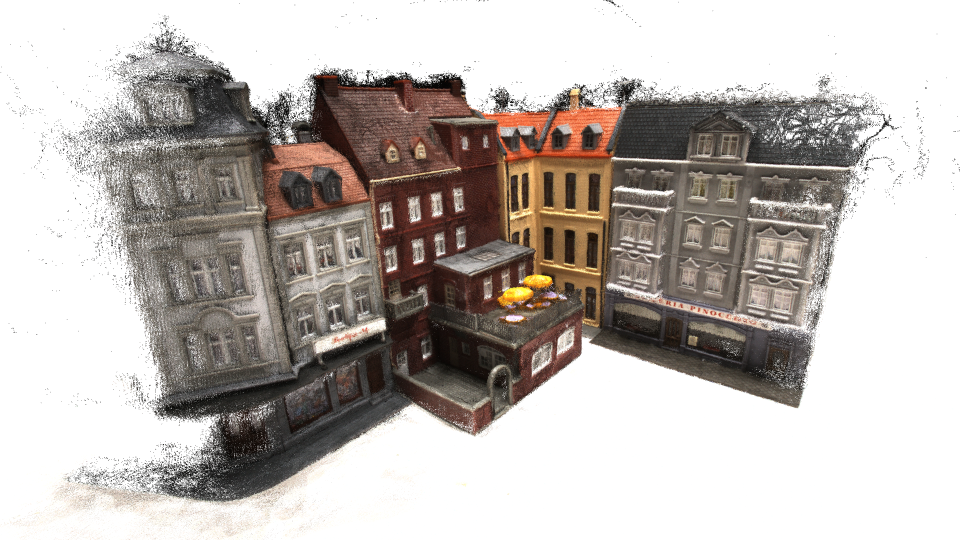}}  \\
         \fbox{\includegraphics[trim={400 0 400 0},clip,height=\imh, width=\imw, keepaspectratio]{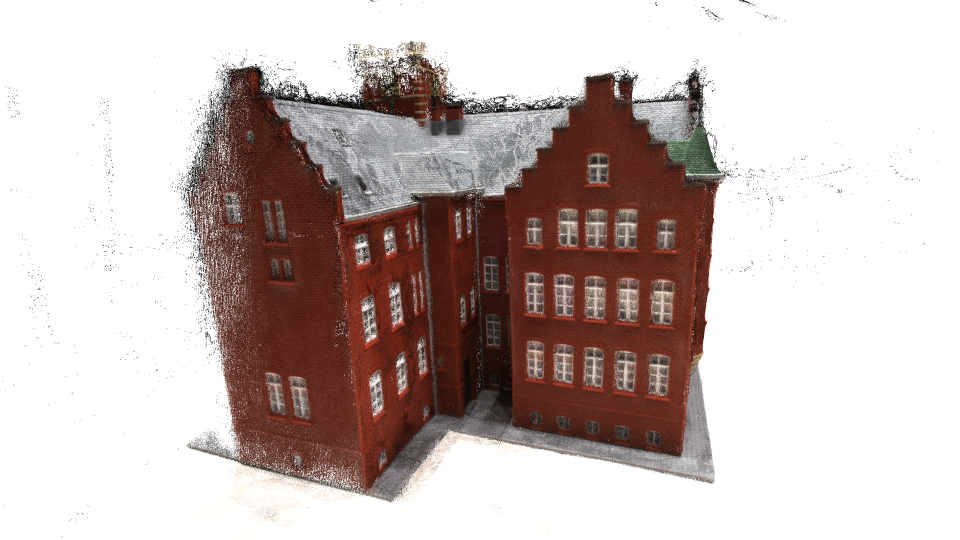}} &
         \fbox{\includegraphics[trim={650 200 450 0},clip,height=\imh, width=\imw,keepaspectratio]{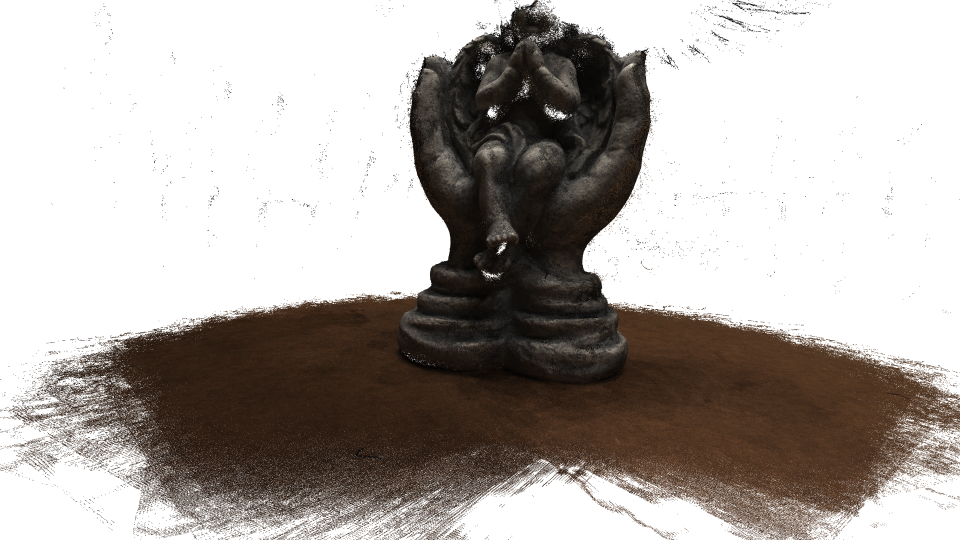}}  &
        \fbox{\includegraphics[trim={600 100 500 50},clip,height=\imh, width=\imw,keepaspectratio]{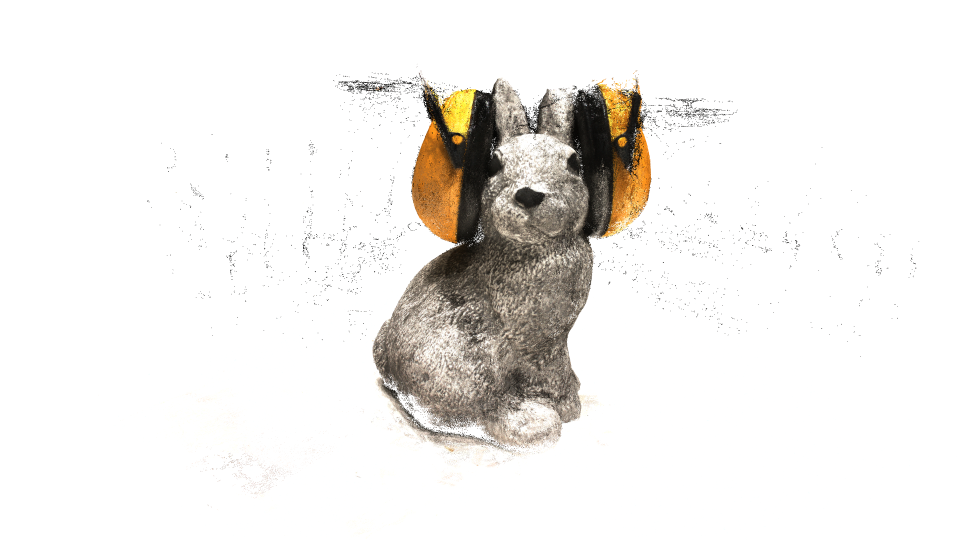}}  \\
         \fbox{\includegraphics[trim={100 0 100 100},clip,height=\imh, width=\imw, keepaspectratio]{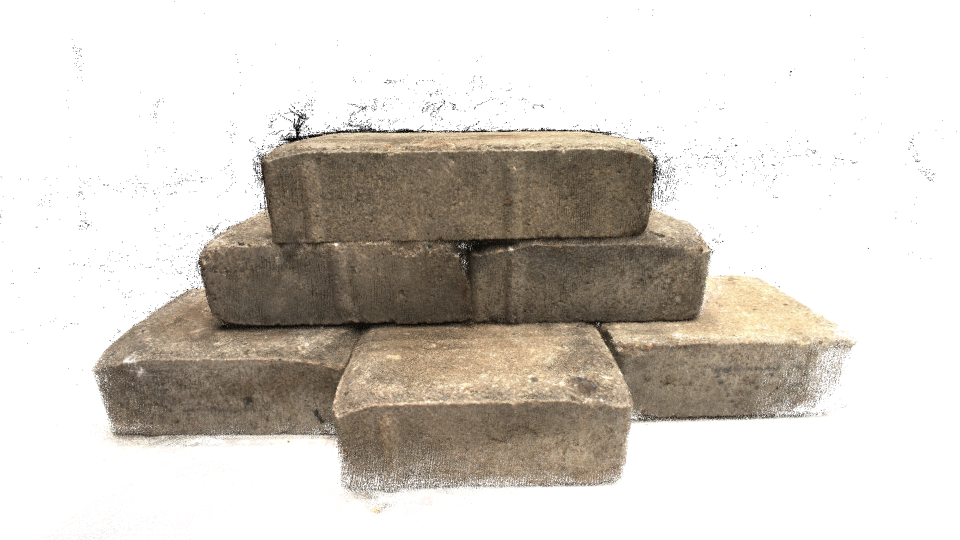}} &
        \fbox{\includegraphics[trim={500 0 100 50},clip,height=\imh, width=\imw, keepaspectratio]{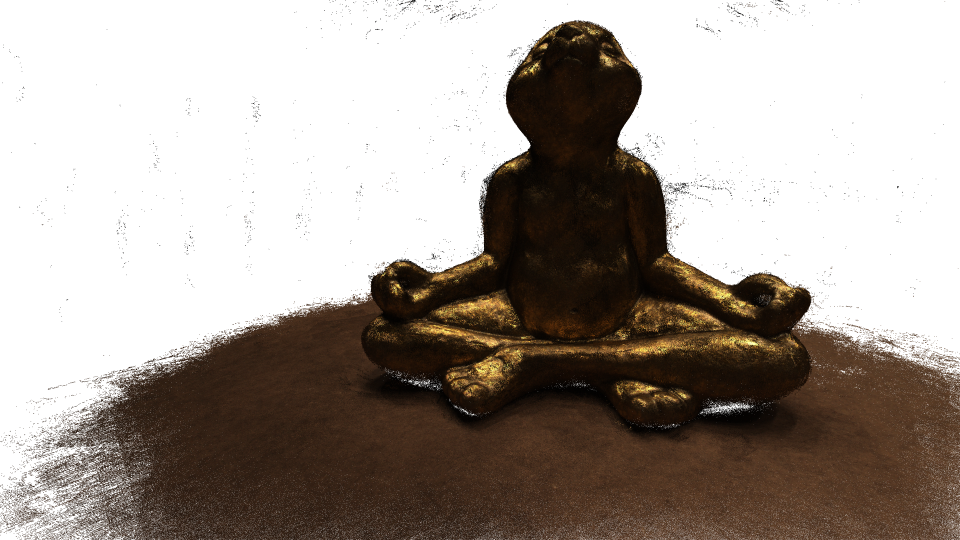}} &
     \fbox{\includegraphics[trim={100 0 100 50},clip,height=\imh, width=\imw, keepaspectratio]{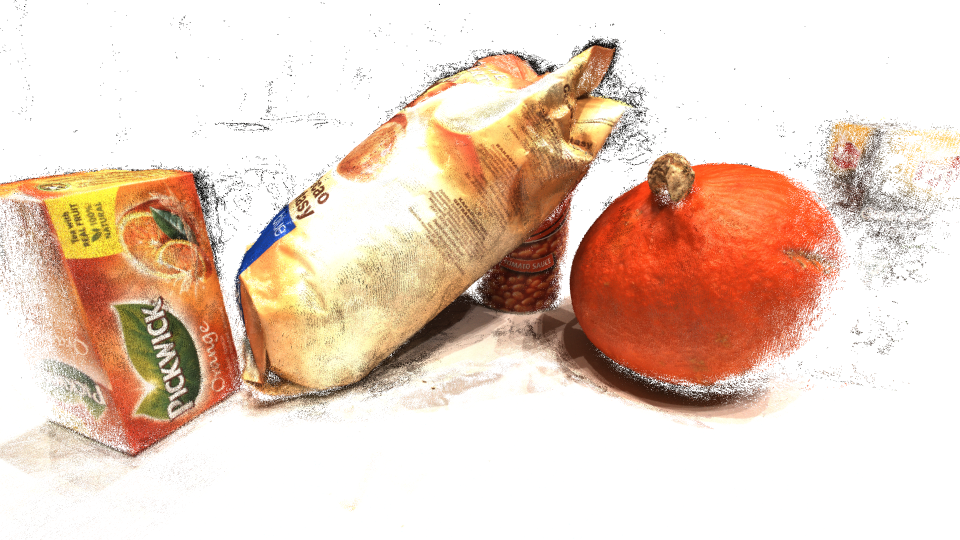}}\\
	 \end{tabular}
     \vspace{-5pt}
     \caption{Qualitative 3D reconstruction results on the DTU test set. We use 4 reference views during the evaluation. The results are obtained from fusing multi-view depth prediction using the tool provided by PatchMatchNet~\cite{wang2021patchmatchnet}.}
     \label{fig:visualization:dtu}\vspace{-1mm}
   \end{figure*}
\endgroup
